# Supplementary material for: GAMA/DEVILS: Cosmic star formation and AGN activity over 12.5 billion years
Source: arXiv:2306.16040 source file (2023-06-28)
Supplement: Supplementary file 1 [file Appendices.tex]

\begin{figure*}
    \centering
    \includegraphics[width = \textwidth]{Figures/MASS-Hists/Stellar-Mass-Distributions-Splice.pdf}
    \caption{Splice}
    \label{fig:my_label}
\end{figure*}
\begin{figure*}
    \centering
    \includegraphics[width = \textwidth]{Figures/MASS-Hists/Stellar-Mass-Distributions-AGN.pdf}
    \caption{AGN only}
    \label{fig:my_label}
\end{figure*}
\begin{figure*}
    \centering
    \includegraphics[width = \textwidth]{Figures/MASS-Hists/Stellar-Mass-Distributions-noAGN.pdf}
    \caption{no AGN}
    \label{fig:my_label}
\end{figure*}
\begin{figure*}
    \centering
    \includegraphics[width = \textwidth]{Figures/MASS-Hists/Phi-Stellar-Mass-Distributions-Splice.pdf}
    \caption{Splice}
    \label{fig:my_label}
\end{figure*}
\begin{figure*}
    \centering
    \includegraphics[width = \textwidth]{Figures/MASS-Hists/Phi-Stellar-Mass-Distributions-AGN.pdf}
    \caption{AGn only}
    \label{fig:my_label}
\end{figure*}
\begin{figure*}
    \centering
    \includegraphics[width = \textwidth]{Figures/MASS-Hists/Phi-Stellar-Mass-Distributions-noAGN.pdf}
    \caption{no AGN}
    \label{fig:my_label}
\end{figure*}

\newpage
\begin{figure*}
    \centering
    \includegraphics[width = \textwidth]{Figures/SFR-Hists/SFR-Distributions-Splice.pdf}
    \caption{Splice}
    \label{fig:my_label}
\end{figure*}
\begin{figure*}
    \centering
    \includegraphics[width = \textwidth]{Figures/SFR-Hists/SFR-Distributions-AGN.pdf}
    \caption{AGN only}
    \label{fig:my_label}
\end{figure*}
\begin{figure*}
    \centering
    \includegraphics[width = \textwidth]{Figures/SFR-Hists/SFR-Distributions-noAGN.pdf}
    \caption{no AGN}
    \label{fig:my_label}
\end{figure*}
\begin{figure*}
    \centering
    \includegraphics[width = \textwidth]{Figures/SFR-Hists/Phi-SFR-Distributions-Splice.pdf}
    \caption{Splice}
    \label{fig:my_label}
\end{figure*}
\begin{figure*}
    \centering
    \includegraphics[width = \textwidth]{Figures/SFR-Hists/Phi-SFR-Distributions-AGN.pdf}
    \caption{AGn only}
    \label{fig:my_label}
\end{figure*}
\begin{figure*}
    \centering
    \includegraphics[width = \textwidth]{Figures/SFR-Hists/Phi-SFR-Distributions-noAGN.pdf}
    \caption{no AGN}
    \label{fig:my_label}
\end{figure*}

\newpage
\begin{figure*}
    \centering
    \includegraphics[width = \textwidth]{Figures/AGN-DATASETS/AGN-Super-Datasets-All-AGN.pdf}
\end{figure*}
\begin{figure*}
    \centering
    \includegraphics[width = \textwidth]{Figures/AGN-DATASETS/AGN-Super-Datasets-AGN_LB.pdf.pdf}
\end{figure*}
\begin{figure*}
    \centering
    \includegraphics[width = \textwidth]{Figures/AGN-DATASETS/AGN-Super-Datasets-AGN_0.pdf}
\end{figure*}
\begin{figure*}
    \centering
    \includegraphics[width = \textwidth]{Figures/AGN-DATASETS/PhixAGN-Super-Datasets-All-AGN.pdf}
\end{figure*}
\begin{figure*}
    \centering
    \includegraphics[width = \textwidth]{Figures/AGN-DATASETS/PhixAGN-Super-Datasets-AGN_LB.pdf}
\end{figure*}
\begin{figure*}
    \centering
    \includegraphics[width = \textwidth]{Figures/AGN-DATASETS/PhixAGN-Super-Datasets-AGN_0.pdf}
\end{figure*}
